# Supplementary material for: Fully kinetic model of plasma expansion in a magnetic nozzle
Source: arXiv:2111.11698 source file (2022-02-22)
Supplement: Supplementary file 1 [file appendix_MM.tex]

%\appendix
%\section*{Appendix. Derivation of the Robin boundary condition}
%\setcounter{section}{1}
%Generally, the electric potential is equal to the sum of the point charges' individual potentials of the $N_p$ charged particles with positions $\mathbf{r}_p$. Consider the potential very far from the localised charge distribution of the plume; it resembles a total point-like charge. Griffiths \cite{b:griffiths2013} provides a multipole expansion for the approximate potentials at large distances $\mathbf{r}$ from a localised charge distribution, which is modified here to the discrete form and relative to the potential at infinity,


%\begin{equation}
%\phi(\mathbf{r}) = \frac{1}{4\pi\epsilon_0}\sum_{n=0}^\infty\frac{1}{|\mathbf{r}|^{n+1}}\sum^{N_p}_{p=1} (\mathbf{r}_p)^n {P}_n(\cos\theta_p)q_p + \phi_\infty,
%\end{equation}

%where ${P}_n$ is the Legendre polynomial operator and $\theta_p$ is the angle between $\mathbf{r}$ and $\mathbf{r}_p$. This is the multipole expansion of $\phi$ in powers of $1/|\mathbf{r}|$. The first term ($n=0$) is the monopole contribution $1/|\mathbf{r}|$; the second ($n=1$) is the dipole contribution $1/|\mathbf{r}|^2$; the third is quadropole; the fourth octopole; and so on.

%Equation A.1 is exact, but it is useful primarily as an approximation scheme. The lowest non-zero term in the expansion provides the approximate potential at large $\mathbf{r}$. At very large $\mathbf{r}$, the expansion is dominated by the monopole term and the potential far from the plasma source is, to good approximation,  

%\begin{equation}
%\phi(\mathbf{r}) = \frac{1}{4\pi\epsilon_0}\frac{1}{|\mathbf{r}|}\sum^{N_p}_{p=1}q_p + \phi_\infty,
%\end{equation}

%where $\sum^{N_p}_{n=1}q_i$ is the total net charge in the plume, which, for a partially confined plasma, is not null (plasma is non-neutral in the equivalent wall sheath). Equation A.2 is the standard $1/r$ monopole decay into vacuum. Taking the first derivative of the potential in Equation A.2 gives,

%\begin{equation}
%\nabla\phi(\mathbf{r}) = -\frac{1}{4\pi\epsilon_0}\frac{1}{|\mathbf{r}|^2}\sum^{N_p}_{p=1}q_p
%\end{equation}

%Substituting Equation A.2 into Equation A.3 then allows a formal solution to be found between the electric field and potential at large $\mathbf{r}$,

%\begin{equation}
%-\nabla\phi(\mathbf{r}) = \frac{1}{|\mathbf{r}|}\left(\phi(\mathbf{r})-\phi_\infty\right),
%\end{equation}

%or, in terms of the potential gradient along a unit normal vector $\hat{\mathbf{n}}$

%\begin{equation}
%  \frac{\partial\phi}{\partial\hat{\mathbf{n}}}+\frac{\hat{\mathbf{n}}\cdot{\mathbf{r}}}{\mathbf{r}\cdot\mathbf{r}}\left(\phi(\mathbf{r})-\phi_\infty\right) = 0
%\end{equation}
